# Supplementary material for: Same Error, Different Function: The Optimizer as an Implicit Prior in Financial Time Series
Source: arXiv:2603.02620 source file (2026-10-27)
Supplement: Supplementary file 1 [file table_appendix_vol_sorted_summary.tex]

\begin{tabular}{llllrrrrr}
\toprule
model & family & optimizer & quintile & ann\_ret & ann\_vol & sharpe & max\_dd & turnover \\
\midrule
pred\_cnn\_100\_sgd & CNN & SGD & Q1 & 0.121000 & 0.173000 & 0.700000 & -0.502000 & 0.065000 \\
pred\_cnn\_100\_muon & CNN & Muon & Q1 & 0.120000 & 0.173000 & 0.691000 & -0.493000 & 0.126000 \\
pred\_mlp\_100\_muon & MLP & Muon & Q1 & 0.118000 & 0.173000 & 0.682000 & -0.496000 & 0.142000 \\
pred\_lstm\_100\_sgd & LSTM & SGD & Q1 & 0.118000 & 0.173000 & 0.682000 & -0.500000 & 0.154000 \\
pred\_lstm\_100\_muon & LSTM & Muon & Q1 & 0.117000 & 0.173000 & 0.676000 & -0.511000 & 0.174000 \\
pred\_mlp\_100\_adam & MLP & Adam & Q1 & 0.120000 & 0.173000 & 0.690000 & -0.502000 & 0.179000 \\
pred\_cnn\_100\_adam & CNN & Adam & Q1 & 0.117000 & 0.173000 & 0.678000 & -0.505000 & 0.183000 \\
pred\_lstm\_100\_adam & LSTM & Adam & Q1 & 0.118000 & 0.174000 & 0.680000 & -0.502000 & 0.186000 \\
ols & Linear & NA & Q1 & 0.119000 & 0.173000 & 0.686000 & -0.498000 & 0.192000 \\
pred\_mlp\_100\_sgd & MLP & SGD & Q1 & 0.118000 & 0.173000 & 0.682000 & -0.508000 & 0.195000 \\
lasso\_0.05 & Linear & NA & Q1 & 0.118000 & 0.173000 & 0.680000 & -0.500000 & 0.205000 \\
pred\_cnn\_100\_sgd & CNN & SGD & Q5 & 0.123000 & 0.283000 & 0.437000 & -0.703000 & 0.057000 \\
pred\_cnn\_100\_muon & CNN & Muon & Q5 & 0.128000 & 0.282000 & 0.454000 & -0.683000 & 0.095000 \\
pred\_mlp\_100\_muon & MLP & Muon & Q5 & 0.125000 & 0.283000 & 0.443000 & -0.693000 & 0.098000 \\
pred\_lstm\_100\_sgd & LSTM & SGD & Q5 & 0.123000 & 0.281000 & 0.438000 & -0.677000 & 0.123000 \\
pred\_lstm\_100\_muon & LSTM & Muon & Q5 & 0.126000 & 0.281000 & 0.449000 & -0.699000 & 0.137000 \\
ols & Linear & NA & Q5 & 0.125000 & 0.282000 & 0.442000 & -0.693000 & 0.140000 \\
pred\_mlp\_100\_adam & MLP & Adam & Q5 & 0.127000 & 0.281000 & 0.453000 & -0.684000 & 0.140000 \\
pred\_cnn\_100\_adam & CNN & Adam & Q5 & 0.126000 & 0.281000 & 0.448000 & -0.694000 & 0.146000 \\
pred\_lstm\_100\_adam & LSTM & Adam & Q5 & 0.131000 & 0.280000 & 0.466000 & -0.677000 & 0.149000 \\
lasso\_0.05 & Linear & NA & Q5 & 0.128000 & 0.281000 & 0.455000 & -0.683000 & 0.151000 \\
pred\_mlp\_100\_sgd & MLP & SGD & Q5 & 0.128000 & 0.280000 & 0.457000 & -0.697000 & 0.151000 \\
\bottomrule
\end{tabular}
