# Supplementary material for: Same Error, Different Function: The Optimizer as an Implicit Prior in Financial Time Series
Source: arXiv:2603.02620 source file (2026-10-27)
Supplement: Supplementary file 2 [file table_vol_regime_pred_lstm_100_sgd.tex]

\begin{tabular}{lrrrr}
\toprule
 & Market (Timed) & Market (BH) & Q1 (Timed) & Q1 (BH) \\
\midrule
AnnRet & 0.090000 & 0.123000 & 0.083000 & 0.119000 \\
AnnVol & 0.114000 & 0.198000 & 0.088000 & 0.174000 \\
Sharpe & 0.785000 & 0.623000 & 0.950000 & 0.685000 \\
MaxDD & -0.342000 & -0.554000 & -0.254000 & -0.500000 \\
\bottomrule
\end{tabular}
